# Supplementary material for: Smart Quantum Technologies using Photons
Source: arXiv:2103.07081 source file (2021-05-02)
Supplement: Supplementary file 1 [file appendix_reuse.tex]

\section{OSA Continuum, OSA Publishing}
\label{ape1}
\begin{figure}[ht!]
    \includegraphics[width=0.94\textwidth]{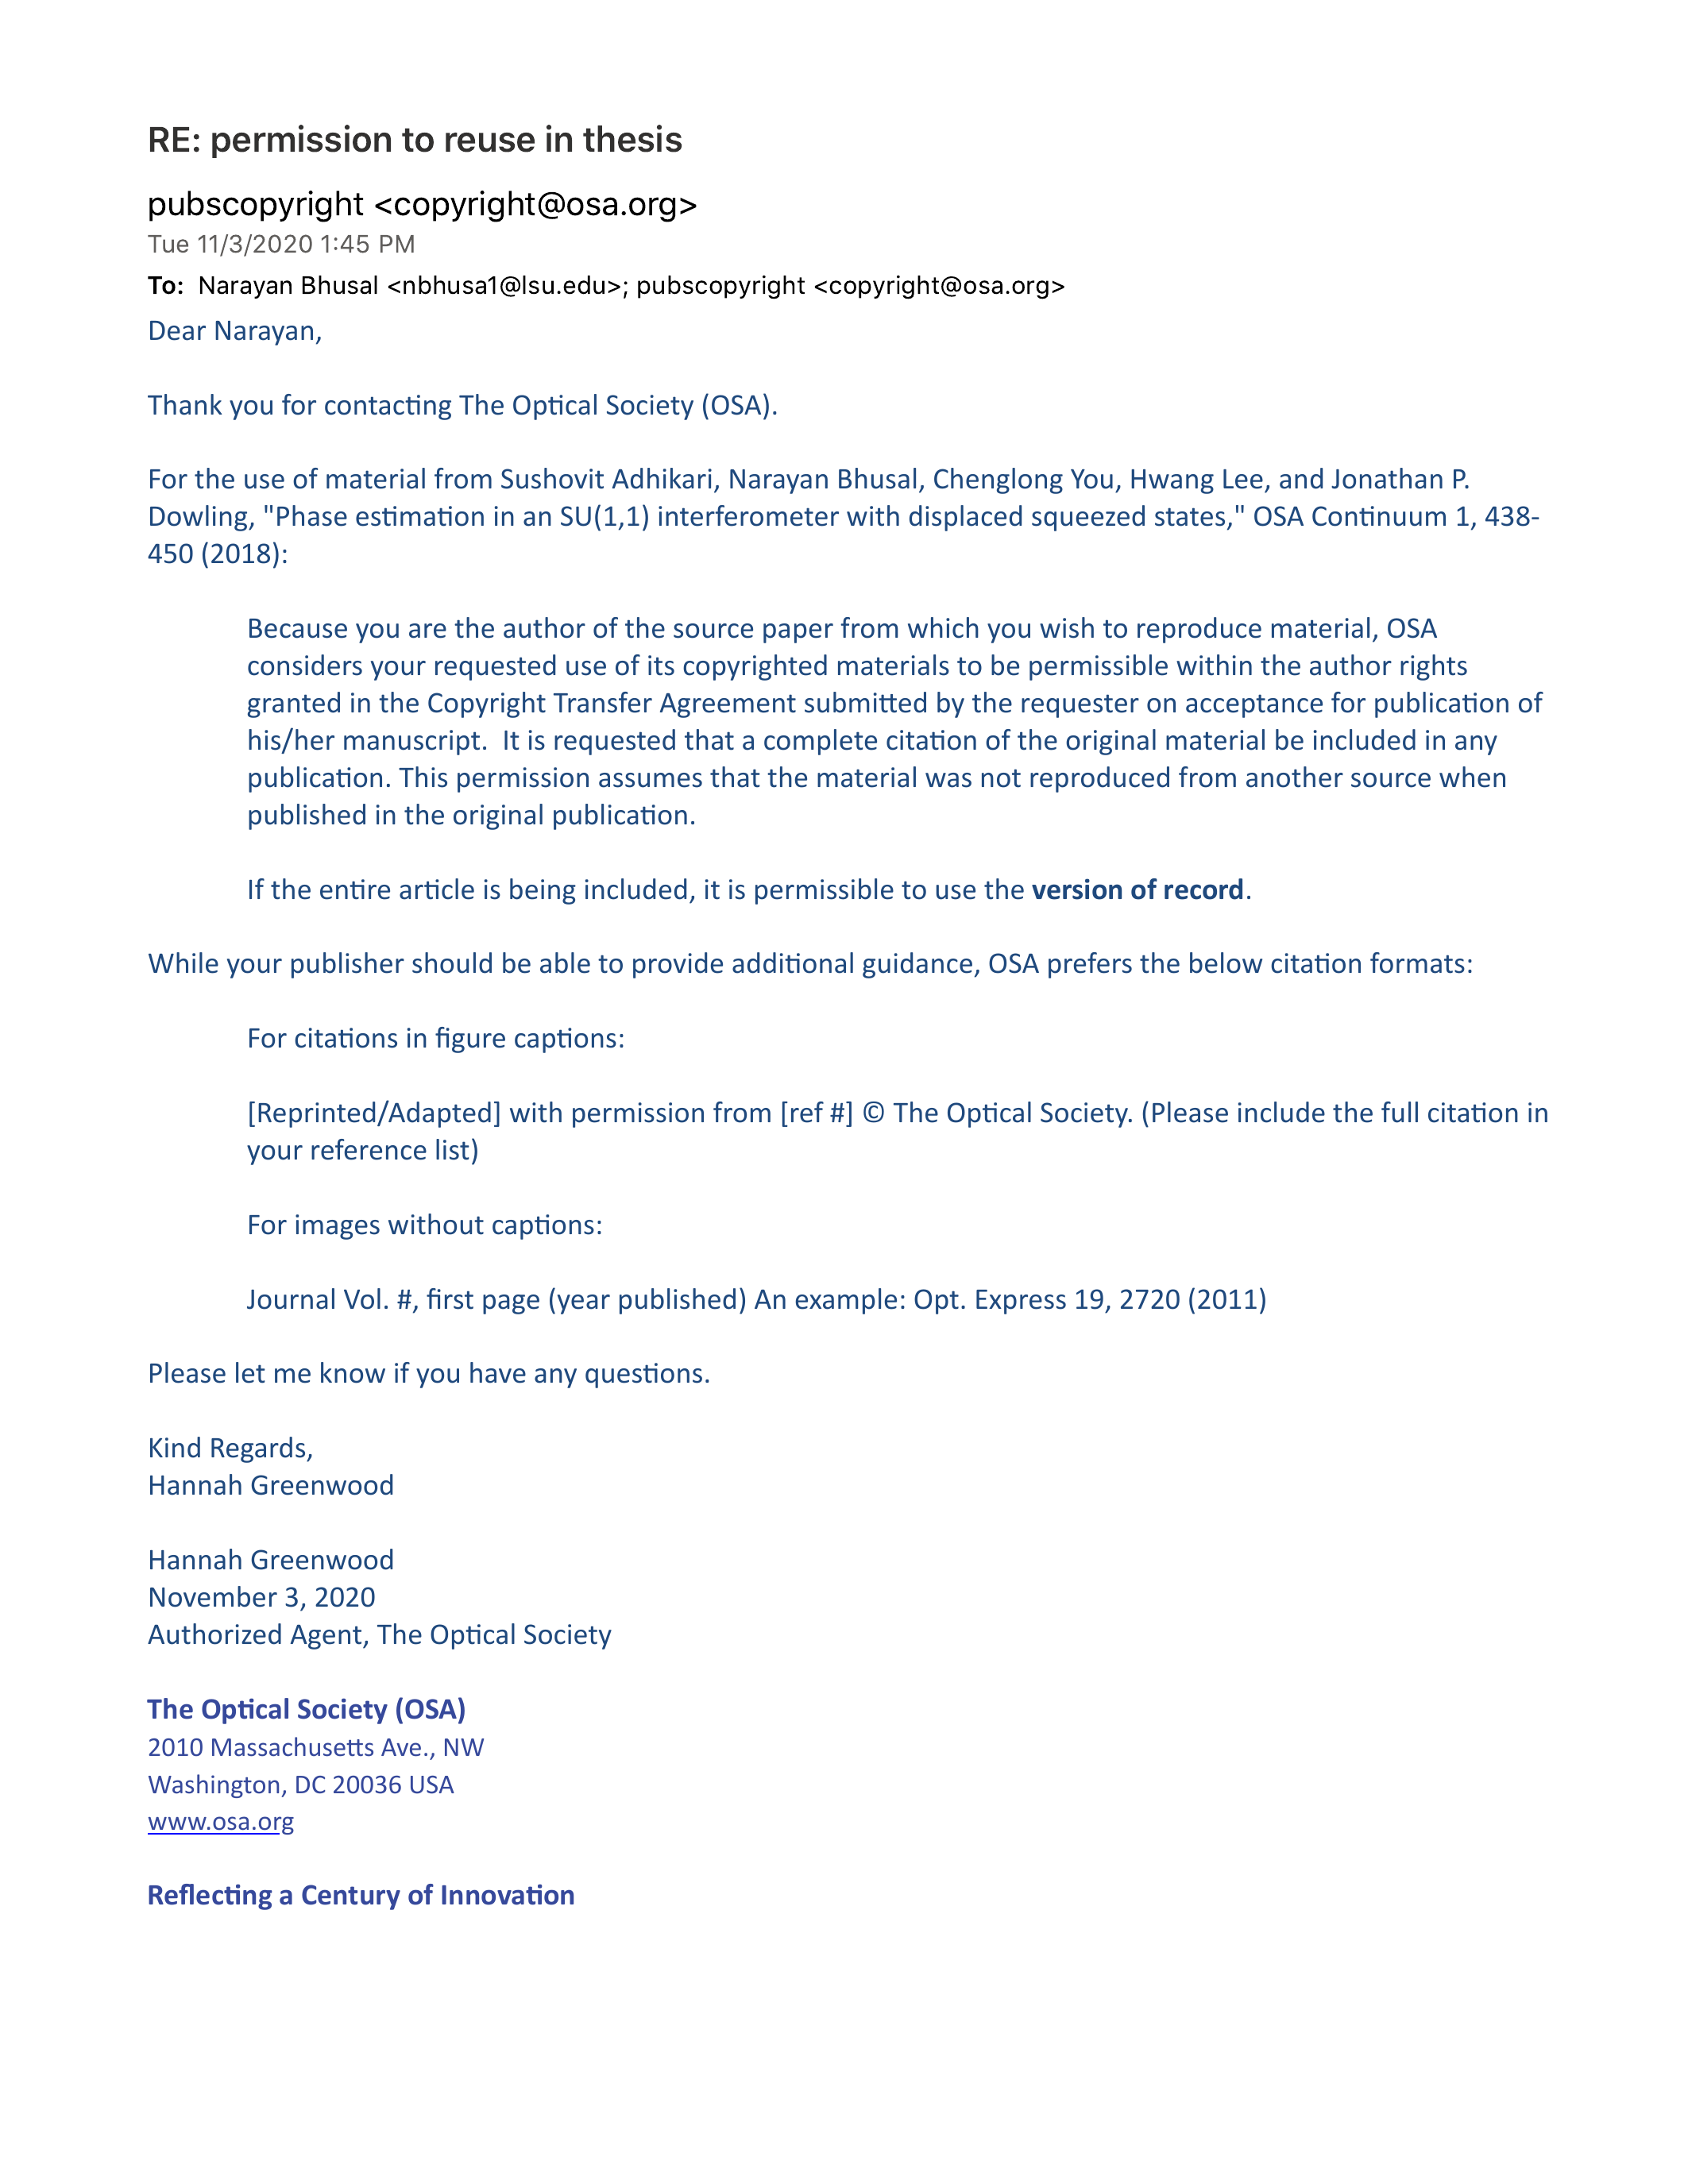}
\end{figure}

\section{Physical Review Letters, APS Publishing}
\vspace{6mm}
\label{ape2}
\noindent\href{https://journals.aps.org/copyrightFAQ.html#thesis}{Click here to see the details on publisher's website!}

\vspace{6mm}
\noindent\textbf{As the author of an APS-published article, may I include my article or a portion of my article in my thesis or dissertation?}
\vspace{6mm}

\noindent Yes, the author has the right to use the article or a portion of the article in a thesis or dissertation without requesting permission from APS, provided the bibliographic citation and the APS copyright credit line are given on the appropriate pages.
\vspace{6mm}

\noindent\textbf{As the author of an APS-published article, may I use figures, tables, graphs, etc. in future publications?}
\vspace{6mm}

\noindent Yes, as the author you have the right to use figures, tables, graphs, etc. in subsequent publications using files prepared and formatted by you or the APS-prepared versions. The appropriate bibliographic citation must be included.
\vspace{6mm}

\noindent \textbf{As the author of an APS-published article, may I give permission to a colleague or third party to republish all or part of the article in a print publication?}
\vspace{6mm}

\noindent Yes, as the author you may grant permission to third parties to republish print versions of the article provided the APS-published version (e.g., the PDF from the online journal, or a copy of the article from the print journal) is not used for this purpose. The article may not be published in another journal, and the third party may not charge a fee. The appropriate bibliographic citation and notice of the APS copyright must be included.

\pagebreak
\section{Applied Physics Reviews, AIP Publishing}
\label{ape3}
\vspace{6mm}
\noindent\href{https://publishing.aip.org/resources/researchers/rights-and-permissions/permissions/}{Click here to see the details on publisher's website!}
\vspace{2mm}

\noindent Authors do not need permission from AIP Publishing to:
\vspace{2mm}
\begin{itemize}
\item quote from a publication (please include the material in quotation marks and provide the customary acknowledgment of the source)
\item reuse any materials that are licensed under a Creative Commons CC BY license (please format your credit line: “Author names, Journal Titles, Vol.\#, Article ID\#, Year of Publication; licensed under a Creative Commons Attribution (CC BY) license.”)
\item \textbf{reuse your own AIP Publishing article in your thesis or dissertation (please format your credit line: “Reproduced from [FULL CITATION], with the permission of AIP Publishing”)}
\item reuse content that appears in an AIP Publishing journal for republication in another AIP Publishing journal (please format your credit line: “Reproduced from [FULL CITATION], with the permission of AIP Publishing”)
\item make multiple copies of articles–although you must contact the Copyright Clearance Center (CCC) at www.copyright.com to do this.
\end{itemize}
\pagebreak

\section{Advanced Quantum Technologies, Wiley}
\label{ape4}
\vspace{6mm}
\noindent\href{https://authorservices.wiley.com/author-resources/Journal-Authors/Promotion/article-sharing-policy.html}{Click here to see the details on publisher's website!}
\vspace{2mm}

\noindent \textbf{For Authors:}

\noindent There are ways of sharing your article at every stage of publication and these are detailed below. You may also share any version of your article with individual colleagues and students if you are asked for a copy, as part of teaching and training at your institution (excluding open online sharing), and as part of a grant application, \textbf{submission of thesis, or doctorate}. For public sharing of your article please see the relevant sections below.

\begin{figure}[ht!]
    \centering
    \includegraphics[width=0.75\textwidth]{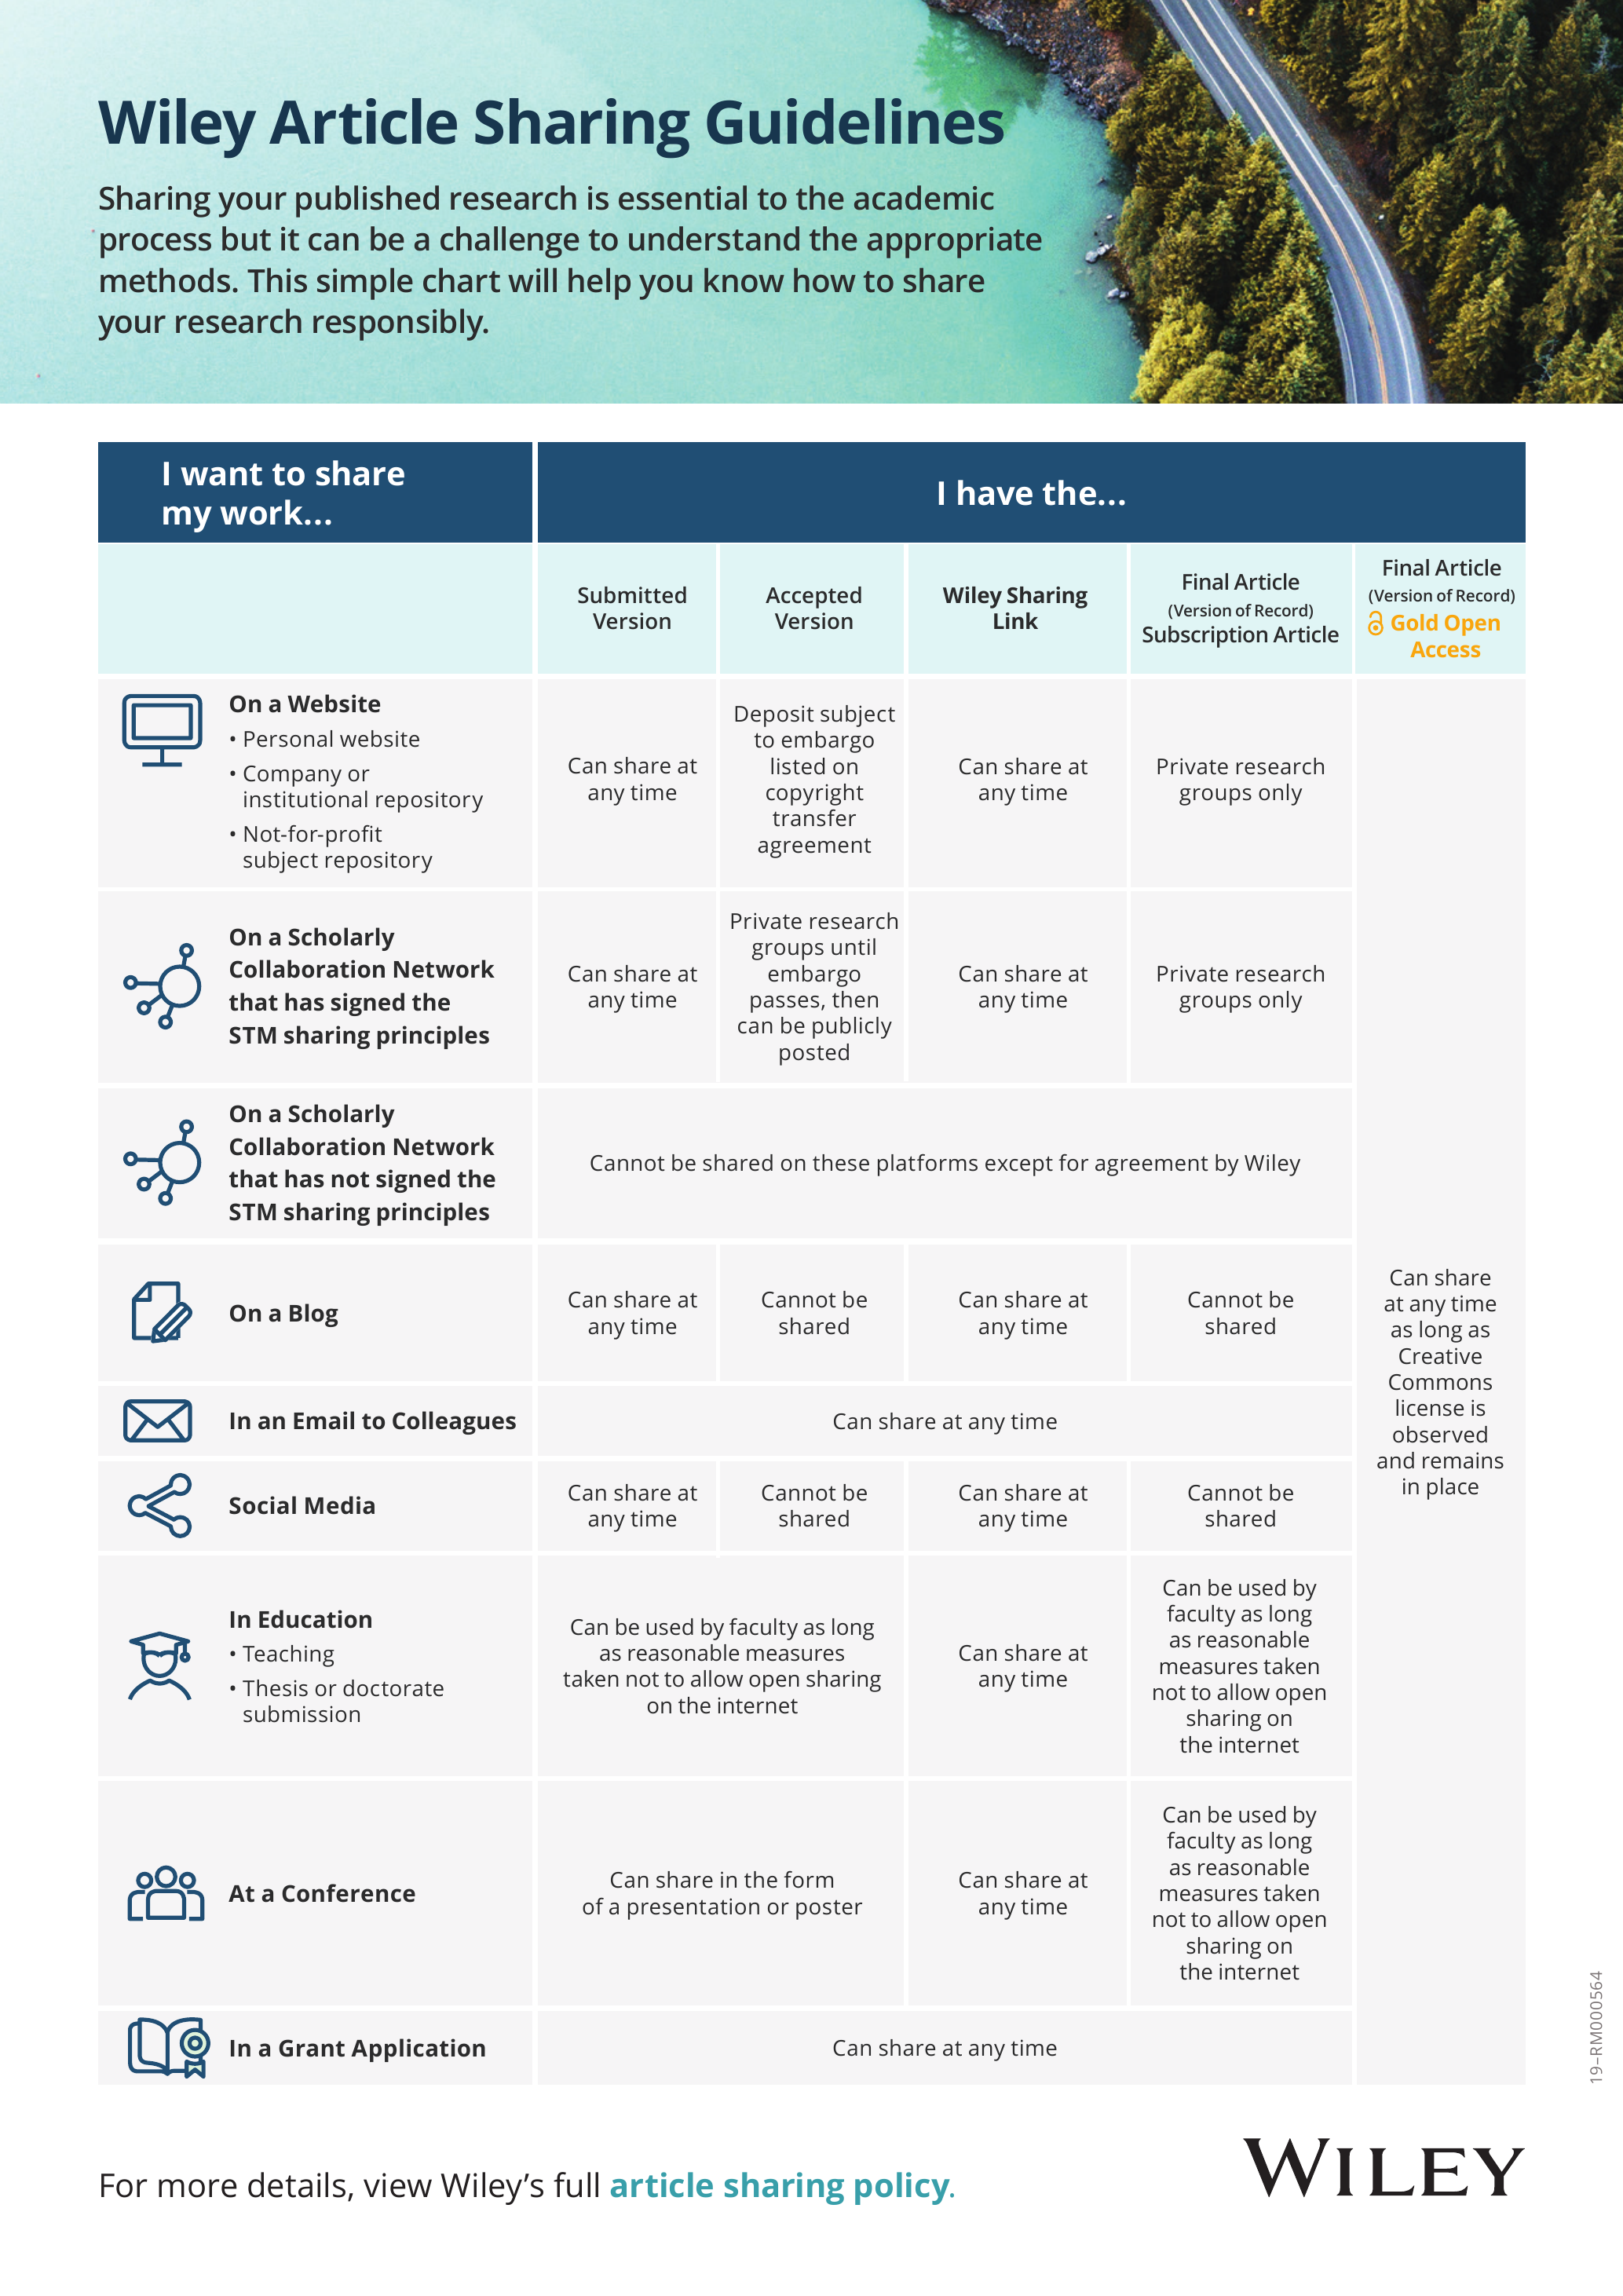}
\end{figure}
